# Supplementary material for: Spin-orbit splitting and effective masses in p-type GaAs two-dimensional hole gases
Source: arXiv:1310.7638 source file (2014-02-17)
Supplement: Supplementary file 1 [file Supplementary.pdf]

# Supplementary material: Spin-orbit splitting and effective masses in p-type GaAs two-dimensional hole gases

Fabrizio Nichele,[1,*] Atindra Nath Pal,[1] Roland Winkler,[2] Christian Gerl,[3] Werner Wegscheider,[1] Thomas Ihn,[1] and Klaus Ensslin[1]

[1]*Solid State Physics Laboratory, ETH Zürich - 8093 Zürich, Switzerland*

[2]*Department of Physics, Northern Illinois University, DeKalb, Illinois 60115, USA*

[3]*Universität Regensburg, Universitätsstrasse 31, 93053 Regensburg, Germany*

(Dated: February 7, 2014)

## Abstract

This supplementary material section provides additional data analysis and technical informations. We describe the mathematical procedure adopted to perform the Fourier analysis of the Shubnikov-de Haas oscillations and identify the various peaks present in the power spectrum. We discuss numerical methods commonly used to suppress mathematical artefacts due to the discreteness of the sampled data points. We provide additional data analysis to quantify the strength of spin-orbit interaction in terms of energy splitting between subbands.

## FOURIER ANALYSIS OF THE DATA

Fig. 1 shows a typical magnetoresistance trace measured in our ungated device at a temperature of 80 mK. The longitudinal resistivity $\rho_{xx}$ (blue, left axis) is plotted with the transverse resistivity $\rho_{xy}$ (red, right axis). The low-field longitudinal resistivity as a function of the magnetic field $B$ is described by the Ando formula in the single subband case. The longitudinal resistivity $\rho_{xx}$ oscillates around the classical Drude resistivity $\rho_0$ according to:

$$\rho_{xx}\left(B,T\right) = \rho_0 \left[1 - 2\exp\left(-\frac{\pi}{\omega_c \tau_q}\right) \frac{2\pi^2 k_B T/\hbar\omega_c}{\sinh\left(2\pi^2 k_B T/\hbar\omega_c\right)} \cos\left(2\pi \frac{hn}{2eB}\right)\right], \qquad (1)$$

where $\tau_q$ is the quantum scattering time, $\omega_c$ the cyclotron frequency, $T$ the temperature and $n$ the carrier density. The oscillatory term is given by $\cos\left(2\pi\frac{hn}{2eB}\right)$, and is periodic in units of $1/B$. The carrier density is derived from the periodicity of $\rho_{xx}(1/B)$. If two subbands contribute to transport in parallel, as in our case, then two different oscillating components contribute to the low-field magnetoresistance. Eq. (1) would then contain an additional oscillating term in the rhs square bracket. In such a situation, it is more convenient to plot the power spectrum of $\rho_{xx}(1/B)$ and calculate the subbands densities from the position of the maxima.

In order to transform our data, we used a discrete Fourier transform based on a fast Fourier transform algorithm included in the software Matlab. To suppress eventual numerical artifact originating from the discreteness and finite dimension of the data range, it is common practice in this kind of analysis, to subtract a slowly varying background, pad the data with zeros and multiply them with a smooth windowing function [1]. The subtraction of the slowly varying background suppresses the low frequency contribution in the power spectrum. The resolution of the power spectrum depends on the real space extension of the data points to be transformed. To increase the number of points in the discrete frequency spectrum, we extended the data range with vectors of zeros (ten times longer than the original data). Padding the data with zeros results in a smooth interpolation of the transformed spectrum that does not increase the true resolution. Zero-padding the data does not preclude further analysis. The multiplication of the data with a magnetic field dependent function (also called windowing) corresponds, in the frequency domain, to the convolution between the spectrum of the data and the Fourier transform of the window. The bare selection of a particular range in magnetic field corresponds to window the data

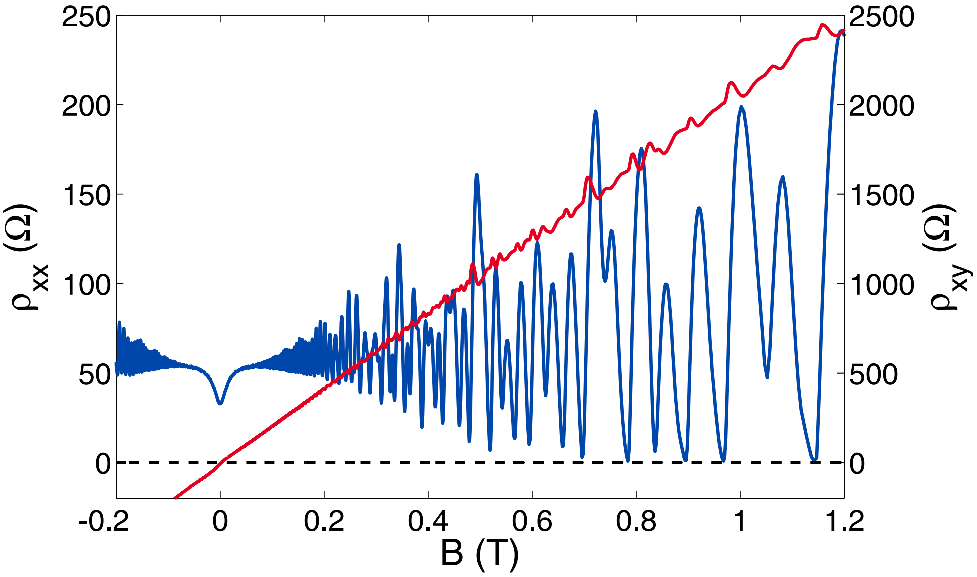


FIG. 1. (color online). Longitudinal resistivity $\rho_{xx}$ (blue) and transverse resistivity $\rho_{xy}$ (red) measured in the ungated sample.

with a rectangular function. This operation creates hard boundaries on the data set to be transformed and, as a consequence, spurious side peaks might appear in the final result. In order to minimize the contribution of the boundaries it is common practice to window the data with a smooth function that minimizes the contribution of the edges. A detailed discussion about the existing windowing functions and their properties goes beyond the scope of this text.

We perform this exemplary analysis in the magnetic field range between 0.2 T and 1.2 T. The procedure described here produces Fig. 1 in our main manuscript, but the quantitative analysis of the effective mass presented in the main manuscript is done in larger intervals of magnetic field. Fig. 2 shows $\rho_{xx}$ (blue) plotted as a function of $1/B$ in the magnetic field range of interest. The data are interpolated with a cubic spline in order to obtain equally spaced points in $1/B$. In our example, we pass from 3101 data points before interpolation, to 41001 points after interpolation. The data interpolation in a newly defined axis where the points are equally spaced is mandatory in order to perform the fast Fourier transform algorithm. We use a least mean square fit of a sixth order polynomial (red curve in Fig. 2) as a slowly varying background to be subtracted from the data. The result of the subtraction is shown in Fig. 3 (blue). The windowing function used for the analysis is the symmetric

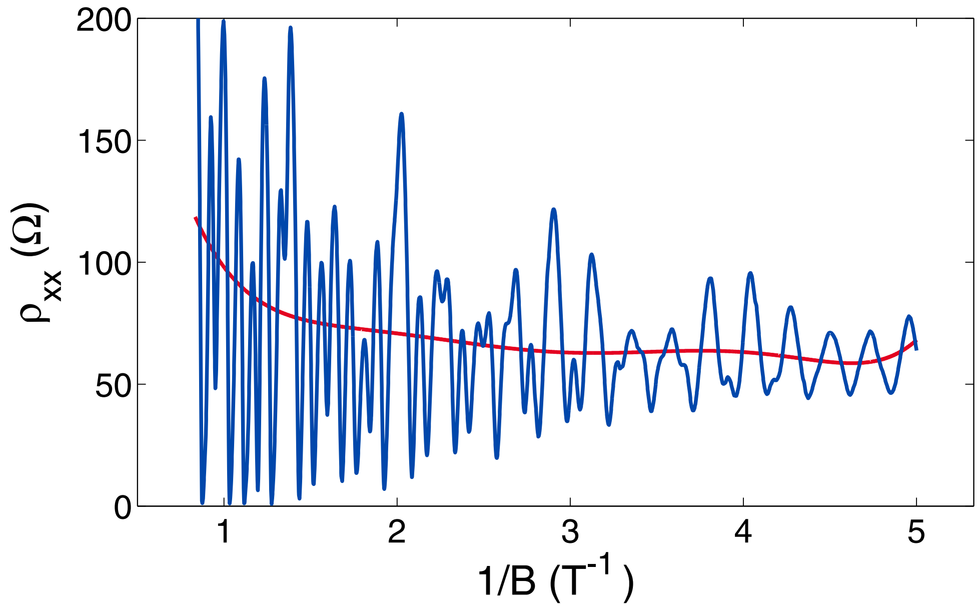


FIG. 2. (color online). Longitudinal resistivity of Fig. 1 plotted as a function of $1/B$ for a magnetic fields between 0.2 T and 1.2 T (blue) and the sixth order polynomial (red) subtracted from the data in order to remove the slowly varying background.

Hamming window (red) [1, 2]. The discrete windowing function consists of the same number N of data points as the data set, and is given by:

$$H(n) = 0.54 - 0.46 \cos\left(2\pi \frac{n}{N}\right), \tag{2}$$

with $0 \leq n \leq N$. Fig. 4 shows the result after windowing the data and padding the result with zeros. The amplitude of the function to be transformed is reduced at the boundaries. We tried different windowing functions, obtaining qualitatively similar results.

Fig. 4 summarizes the analysis results. Subfigures (a) and (b) show the raw data and the corresponding power spectrum respectively in case no particular operation is performed. Subfigures (b) and (c) show the raw data after zero-padding and the corresponding power spectrum respectively. Subfigures (e) and (f) show the raw data after zero-padding and subtraction of a sixth order polynomial and the corresponding power spectrum respectively. Subfigures (g) and (h) show the raw data after zero-padding, subtraction of a sixth order polynomial and multiplication with an Hamming window and the corresponding power spectrum respectively. The spectrum in Fig. 4 (f) shows many side peaks that are absent in Fig. 4 (h), as indicated by the arrows. Windowing is very useful in situations where a specific

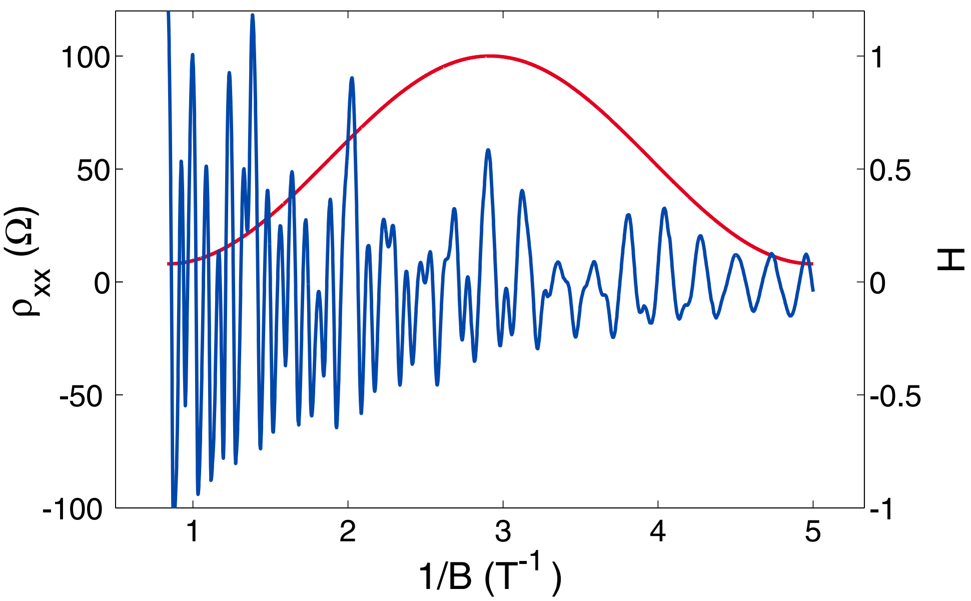


FIG. 3. (color online). Data to be Fourier transformed before windowing (blue) and symmetric Hamming window used for the analysis (red).

frequency component has to be identified from the background. It is important to notice that the relative amplitude of the peaks changes if windowing is performed. For this reason no windowing function is used for Method A in the paper, where an inverse fast Fourier transform is performed on the filtered spectra. For method B the Hamming window is used for both the measured and the calculated data. The operations previously performed leave the amplitude of the peaks of interest unchanged, hence they do not affect the quantitative analysis presented in the main text.

The frequency axis can be directly converted into a (spin-resolved) density axis using the relation $n = fe/h$, as shown in Fig. 5. In the following we will show how all the peaks in the power spectral densities can be consistently interpreted. The highest peak in the power spectrum of Fig. 4 (d) matches the periodicity of the low-field SdH oscillations, visible in Fig. 4 (a) above 4 $T^{-1}$ and can be identified with the first subband oscillations. The total density $n = n_1 + n_2$ is obtained from the Hall slope. The transverse resistivity $\rho_{xy}$ is not linear at small magnetic field due to the presence of the two subbands [3]. We therefore determine the density from the slope of $\rho_{xy}$ between 80 mT and 200 mT, where it corresponds to the total density, and obtain $2.95 \times 10^{15}$ $m^{-2}$. At this density, indicated by the green dot in Fig. 5, the power spectrum shows a peak. The density of the second

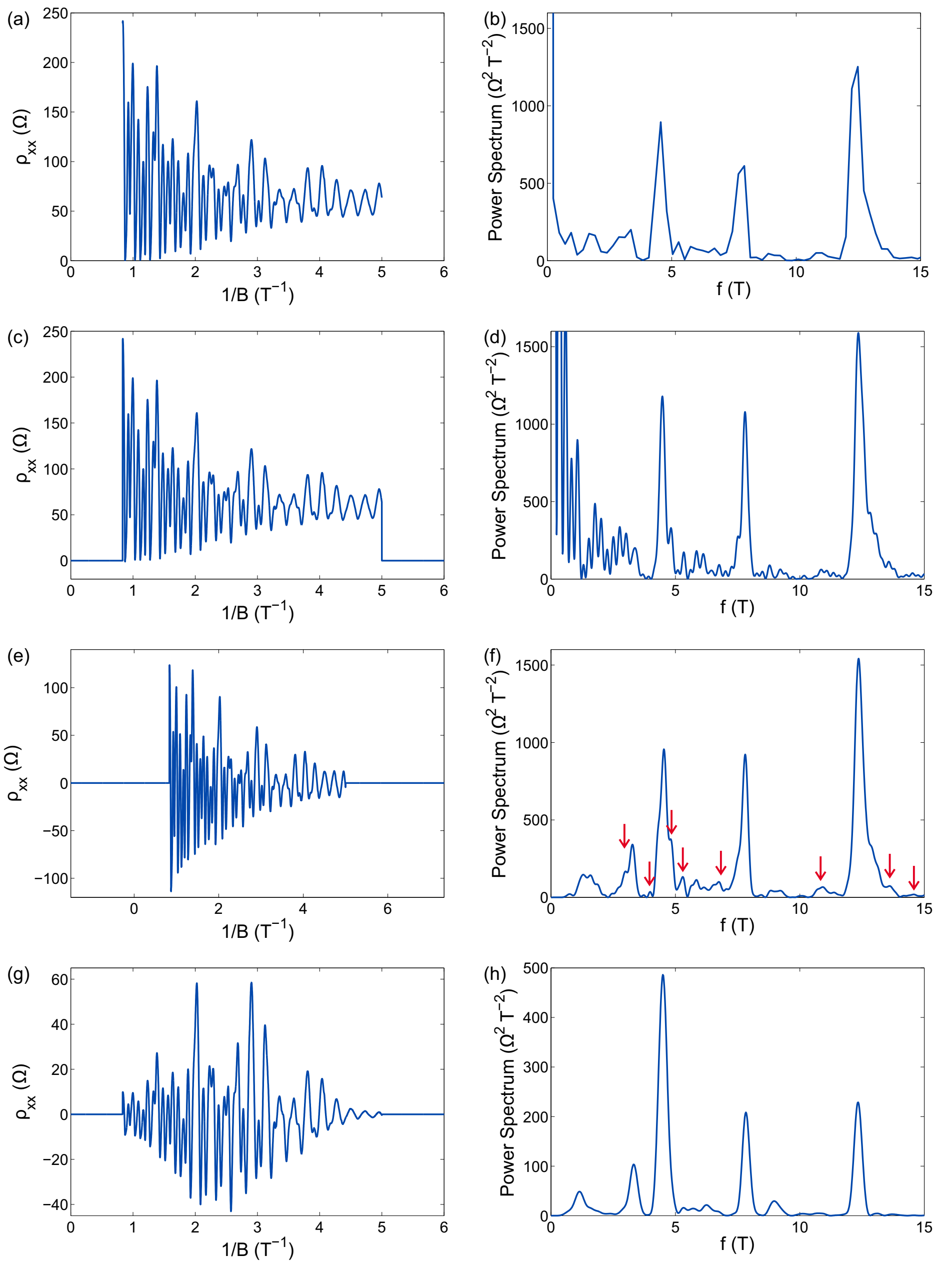


FIG. 4. (color online). (a) Raw data to be transformed, when no particular operation is performed. (b) Power spectrum of the data in (a). (c) Data in (a) after zero-padding. (d) Power spectrum of the data in (c). (e) Data in (c) after subtraction of a sixth order polynomial. (f) Power spectrum of the data in (e), the arrows indicate side peaks that are absent in (h). (g) Data in (e) after multiplication with an Hamming window. (h) Power spectrum of the data in (g). Note that the horizontal extension of the data in (b), (d) and (g) is much larger than what shown in the graphs.

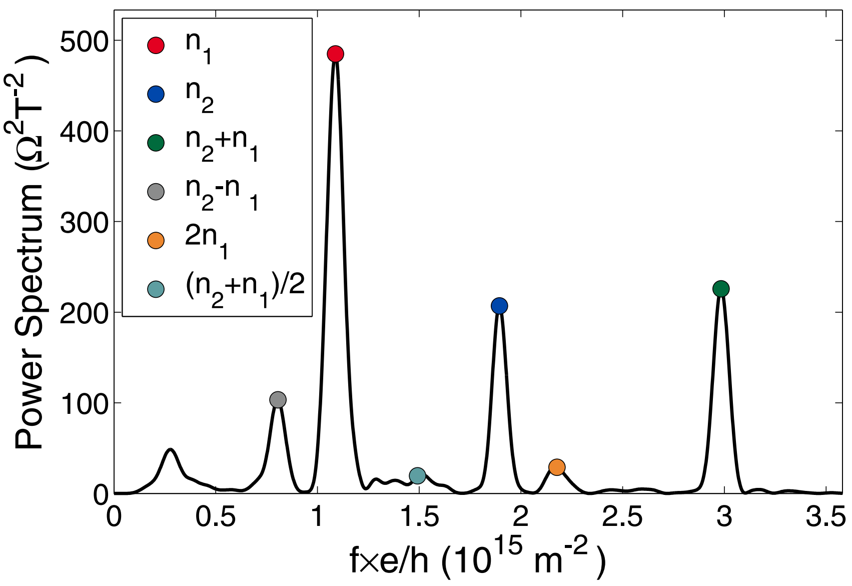


FIG. 5. (color online). Power spectrum as a function of density. The dots indicate the subband densities calculated from the analysis of $\rho_{xx}$ and $\rho_{xy}$. The excellence agreement between the calculated densities and the power spectrum peaks proves consistency for the analysis.

subband is obtained by $n_2 = n - n_1$. The result (blue dot) accurately matches the position of another peak in the spectrum of Fig. 5. The peaks located at frequencies $2n_1$ and $n_2 - n_1$ derive from combinations of $n_1$ and $n_2$. The peak located at a frequency corresponding to the average density $(n_1 + n_2)/2$ cannot be obtained by multiplication of sinusoidal functions. This anomalous peak, already observed in Ref. 4, is interpreted with non-adiabatic effects [5]. The peak visible for a density smaller than $0.5 \times 10^{15} m^{-2}$ is due to a residual of the slowly varying background present in our data after the subtraction of the low order polynomial described above.

## SPIN-ORBIT INTERACTION STRENGHT

Heavy-hole states in p-type GaAs are characterized by an angular momentum $j = 3/2$ in the growth direction, with a $z$ component of the angular momentum of $m = \pm 3/2$. For such a state, it is predicted that the first relevant term in the Hamiltonian containing spin-orbit interaction is not proportional to $k_\parallel$ as in the case of electrons in the conduction band, but proportional to ${k_\parallel}^3$. Consequently, the heavy-hole (HH) in-plane dispersion relation for the

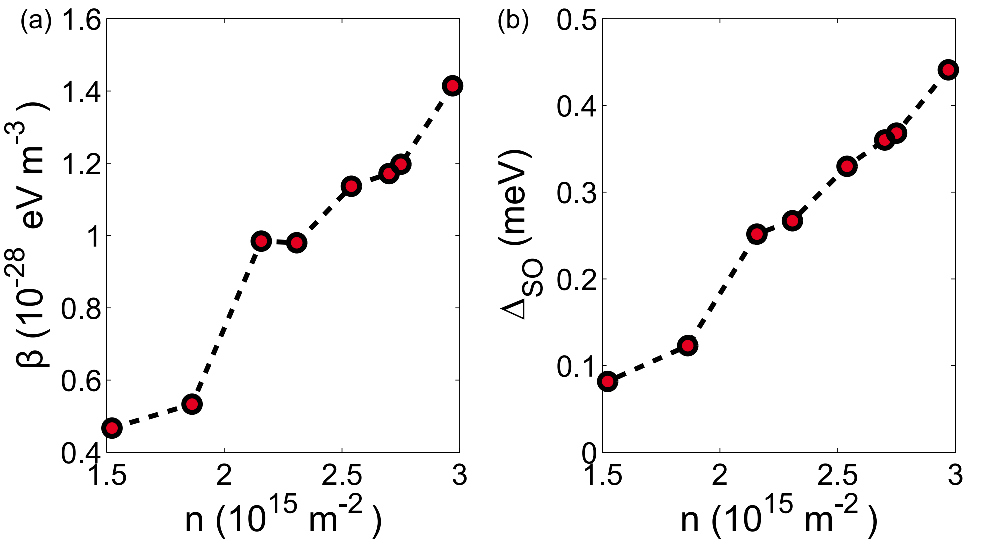


FIG. 6. (color online). Rashba spin-orbit parameter $\beta$ and spin-orbit energy splitting $\Delta_{SO}$ as a function of total density.

case under study is [6]

$$E_{\pm}\left(k_{\parallel}\right) = \langle\mu_h\rangle\, {k_{\parallel}}^2 \pm \beta {k_{\parallel}}^3, \tag{3}$$

where $\langle\mu_h\rangle$ is the average between $\hbar^2/(2m_1)$ and $\hbar^2/(2m_2)$. The Rashba parameter $\beta$ is determined by the subband densities and $\mu_h$ according to

$$\beta = \frac{\langle\mu_h\rangle}{2\sqrt{\pi}} \frac{n_2 - n_1}{n_2^{3/2} + n_1^{3/2}} \tag{4}$$

The energy difference between the spin-split subband is then $\Delta_{SO} = 2\beta {k_{\parallel}}^3$, where $k_{\parallel}$ is taken to be the in-plane Fermi wave vector of the low density subband, defined as $k_1 = \sqrt{4\pi n_1}$. The result of the analysis is shown in Fig. 6. The results show a good gate tunability of the spin-orbit coupling strength and qualitatively match the data reported in [7], where a density independent effective mass was assumed.

* fnichele@phys.ethz.ch; www.nanophys.ethz.ch

[1] J. Tukey, *Advance Seminar on Spectral analysis of time series: proceedings* (Wiley, 1967) pp. 25–46.

[2] F. Harris, *Proceedings of the IEEE*, Proc. IEEE **66**, 51 (1978).

[3] E. Zaremba, Phys. Rev. B **45**, 14143 (1992).

[4] B. Habib, M. Shayegan, and R. Winkler, Semicond. Sci. Technol. **24**, 064002 (2009).

[5] S. Keppeler and R. Winkler, Phys. Rev. Lett. **88**, 046401 (2002).

[6] R. Winkler, *Spin-Orbit Coupling Effects in Two-Dimensional Electron and Hole Systems*, Springer Tracts in Modern Physics, Vol. 191 (Springer-Verlag, Berlin, 2003).

[7] B. Grbić, R. Leturcq, T. Ihn, K. Ensslin, D. Reuter, and A. D. Wieck, Phys. Rev. B **77**, 125312 (2008).
